# Supplementary material for: Optimal Energy Management in Autonomous Power Systems with Probabilistic Security Constraints and Adaptive Frequency Control
Source: arXiv:2208.08953 source file (2022-08-18)
Supplement: Supplementary file 1 [file Appendix_A.tex]

\section{Nomenclature}

\begin{table}[hbt!]
	\centering
    \caption{Nomenclature}
	\label{tab:nomencl}
	\begin{center}
	    \begin{tabular}{cc}
% \caption{Nomenclature.} \label{table:nomencl} \\

    \hline
    \multicolumn{1}{|c|}{\textbf{Description}} & \multicolumn{1}{c|}{\textbf{Symbol}} \\
    \hline 

    \hline \hline

    \multicolumn{2}{c}{\textbf{Optimization problem}} \\
    \hline
           
            continuous time domain index & $t \in \mathcal{R}$ \\
            
            set of lead times (prediction horizon)   & $k \in \mathcal{K}$ \\
            
            set of available synchronous generators & $g \in \mathcal{N}_{g}$ \\
            
            % set of scenarios & $\omega \in \mathcal{N}_{\omega}$ \\
            
            set of system configurations & $j \in \mathcal{J}$ \\
            
            set of samples (scenarios) draws & $\bm{\delta^i} \in \Delta^N$ \\
            
            configuration binary variables  &  $b_j$ \\
            
            GT states &  $\mathbf{x}_{1:N_g}^{gt}$ \\
            
            ESS state &  $\mathbf{x}^{SoC}$ \\
        
            % binary GT status variables &  $x_{g,t}^{gt}$ \\
            
            GT max power &  $\bar{P}^{gt}$ \\
            
            GT min power &  $\underline{P}^{gt}$ \\
            
            GT power &  $\bm{P}_{k}^{gt}$ \\
            
            ESS discharge power &  $P_{k}^{dis}$ \\
            
            ESS charge power &  $P_{k}^{ch}$ \\
            
            ESS power rating &  $\bar{P}^b$ \\
            
            ESS energy rating &  $\bar{E}^b$ \\
            
            % GT turn ON command &  $b_{g}^{gt,on}$ \\
            
            % GT turn OFF command &  $b_{g}^{gt,off}$ \\

            net load forecast &  $\mathbf{\xi}$ \\
            
            % perturbation from UC command &  $P^{b}_{sw}$ \\
            
            net load perturbation &  $P^{b}_{nl}$ \\
            
            % system configuration data matrix &  $\bm{A}_{cf}$ \\
            
            % system configuration startup data matrix &  $\bm{B}^{on}_{cf}$ \\
            
            % system configuration shutdown data matrix &  $\bm{B}^{off}_{cf}$ \\
            
            GT damping coefficient &   $D_g$ \\
            
            ESS damping coefficient &  $D_b$ \\
            
            total system damping coefficient &  $\mathcal{D}$ \\
            
            GT inertia time constant &  $M_g$ \\
            
            ESS virtual inertia time constant &  $M_b$ \\
            
            total system inertia time constant &  $\mathcal{M}$ \\

        \hline
        \hline
        
        	    \end{tabular}
	\end{center}
\end{table}

% \end{longtable}
% \end{center}
