# Supplementary material for: Optimal Energy Management in Autonomous Power Systems with Probabilistic Security Constraints and Adaptive Frequency Control
Source: arXiv:2208.08953 source file (2022-08-18)
Supplement: Supplementary file 2 [file Appendix_B.tex]

\section{}

\begin{equation*}
    \begin{gathered}
        \mathbf{x} =  \left [ x^{SoC}, \mathbf{x}_{1:N_g}^{gt}  \right ]^T
    \end{gathered}
    \label{eq:states_def}
\end{equation*}
\begin{equation*}
    \begin{gathered}
        \mathbf{u} =  \left [ P^{ch}, P^{dis}, u_{1}^{gt,on}, u_{1}^{gt,off},\ldots, u_{N_g}^{gt,on}, u_{N_g}^{gt,off}  \right ]^T
    \end{gathered}
    \label{eq:ctrl_def}
\end{equation*}
\begin{equation*}
    \begin{gathered}
        \bm{b}  = [b_1, \ldots, b_j,  \ldots, b_J]^T
    \end{gathered}
    \label{eq:b_j_vec}
\end{equation*}
\begin{equation*}
    \begin{gathered}
        \bm{\mathcal{D}}   = [\mathcal{D}_1, \ldots, \mathcal{D}_j,  \ldots, \mathcal{D}_J]^T
    \end{gathered}
    \label{eq:D_lin_vec}
\end{equation*}
% \begin{equation*}
%     \begin{gathered}
%         \bm{\mathcal{M}}   = [\mathcal{M}_1, \ldots, \mathcal{M}_j,  \ldots, \mathcal{M}_J]^T
%     \end{gathered}
%     \label{eq:M_lin_vec}
% \end{equation*}
\begin{equation*}
    \begin{gathered}
        \bm{D}_g  = [ D_1 , \ldots, D_g,  \ldots,D_{N_g}]^T
    \end{gathered}
    \label{eq:D_g_vec}
\end{equation*}
% \begin{equation*}
%     \begin{gathered}
%         \bm{M}_g  = [ M_1 , \ldots, M_g,  \ldots,M_{N_g}]^T
%     \end{gathered}
%     \label{eq:M_g_vec}
% \end{equation*}
% \begin{equation*}
%     \begin{gathered}
%         \mathbf{x_+}=\left [\mathbf{x}_{t+0|t},\ldots,\mathbf{x}_{t+k|t},\ldots,\mathbf{x}_{t+\mid \mathcal{K}\mid|t} \right]^T
%     \end{gathered}
%     \label{eq:X_plus}
% \end{equation*}
% \begin{equation*}
%     \begin{gathered}
%         \mathbf{u}=\left [\mathbf{u}_{t+0|t},\ldots,\mathbf{u}_{t+k|t},\ldots,\mathbf{u}_{t+\mid \mathcal{K}\mid|t} \right]^T
%     \end{gathered}
%     \label{eq:U_star}
% \end{equation*}
% \begin{equation*}
%     \begin{gathered}
%         \mathbf{v}=\left [\mathbf{v}_{t+0|t},\ldots,\mathbf{v}_{t+k|t},\ldots,\mathbf{v}_{t+\mid \mathcal{K}\mid|t} \right]^T
%     \end{gathered}
%     \label{eq:V_star}
% \end{equation*}
\begin{equation*}
    \begin{gathered}
        \bm{P}^{b}_{nl}  = [\bm{P}^{b}_{nl,1}, \ldots, \bm{P}^{b}_{nl,j},  \ldots, \bm{P}^{b}_{nl,J}]^T
    \end{gathered}
    \label{eq:P_b__nl_vec}
\end{equation*}
\begin{equation*}
    \begin{gathered}
        \bm{P}_{k}^{gt}  = [ P_{1,k}^{gt} , \ldots, P_{g,k}^{gt},  \ldots, P_{N_g,k}^{gt}]^T
    \end{gathered}
    \label{eq:P_gt_k_vec}
\end{equation*}
% where $p_{g,k}^{gt} = \frac{P_{g,k}^{gt} }{S_b} \; \forall \; g \in \mathcal{N}_g, \; k \in \mathcal{K}$ are the GT powers in per unit.

% KPI definition
% \begin{equation}
%     \begin{gathered}
%      I_f(\mathbf{x}_{+}(t),\mathbf{v}_{0}(t)) =
%       \displaystyle \frac{T_s}{60}  \sum_{t \in T_{t}} \sum_{g \in N_g} \mathcal{F}_{fuel}(P_{0,g}^{gt}(t))P_{0,g}^{gt}(t) + c_{f}^{idle} x_{0,g}^{gt}(t)
%     \end{gathered}
%     \label{eq:kpi_fuel}
% \end{equation}
% \begin{equation}
%     \begin{gathered}
%      I_c(\mathbf{x}_{+}(t),\mathbf{u}_{0}(t),\mathbf{v}_{0}(t)) =
%       I_f(\mathbf{x}_{+}(t),\mathbf{v}_{0}(t))c_f + 
%       \displaystyle c_{gt}^{str} \sum_{t \in T_{t}} \sum_{g \in N_g}  b_{0,g}^{gt,on}(t)
%     \end{gathered}
%     \label{eq:kpi_cost}
% \end{equation}
% \begin{equation}
%     \begin{gathered}
%      I_{sw}(\mathbf{u}_{0}(t)) =
%      \displaystyle  \displaystyle \sum_{t \in T_{t}} \sum_{g \in N_g}  b_{0,g}^{gt,on}(t) + \sum_{t \in T_{t}} \sum_{g \in N_g}  b_{0,g}^{gt,off}(t)
%     \end{gathered}
%     \label{eq:kpi_on_off}
% \end{equation}
% \begin{equation}
%     \begin{gathered}
%      I_{de}(\mathbf{u}_{0}(t),\mathbf{v}_{0}(t)) =
%       \displaystyle \frac{T_s}{60}  \sum_{t \in T_{t}} \sum_{g \in N_g} P_{0,g}^{gt}(t) - \left( P_{0}^{ch}(t)-P_{0}^{dis}(t) \right)-  \xi_{0}(t)
%     \end{gathered}
%     \label{eq:kpi_dump}
% \end{equation}
% \begin{equation}
%     \begin{gathered}
%      I_{dg}(\mathbf{x}_{+}(t),\mathbf{u}_{0}(t)) =
%       \displaystyle  \sum_{t \in T_{t}} D^{cyc}(t)
%     \end{gathered}
%     \label{eq:kpi_deg}
% \end{equation}
